# Supplementary material for: Ges3ViG: Incorporating Pointing Gestures into Language-Based 3D Visual Grounding for Embodied Reference Understanding
Source: arXiv:2504.09623 source file (2025-04-13)
Supplement: Supplementary file 1 [file X_suppl.tex]

\clearpage
\setcounter{page}{1}
\setcounter{figure}{0}
\setcounter{table}{0}
\maketitlesupplementary
\newcommand{\variable}[1]{{\color{blue}$<$#1$>$}}

\appendix
In this supplementary material, we provide additional details about several aspects discussed in the paper. 
To begin, we would like to highlight that our dataset and code is made publicly available. 
Readers can access the code for both \names and the \aug framework, as well as information on downloading the complete \dataset dataset, via \url{https://github.com/AtharvMane/Ges3ViG}.

The following sections elaborate on various components of the \datasetns \ dataset.

\section{Language Description Generation}

In our \aug framework, we introduced a Language Description Generation step designed to augment the original language descriptions in ScanRefer, detailed in Section~\ref{subsec:gemini}. This step augments the verbal descriptions by integrating information about the existence of additional pointing gestures. Specifically, we used Gemini \cite{gemini} to augment the existing verbal descriptions by incorporating this context of the presence of additional pointing gestures. To achieve this, we utilized a carefully designed textual prompt, which we describe in detail below:

\begin{enumerate}
    \item \textbf{Context Paragraph:} Provide a detailed explanation of the task that serves as the context for the LLM.
    \item \textbf{Output Specifications:} Specify clear instructions for the LLM on how to structure its response, including the required format.
    \item \textbf{Query:} The original query sourced from ScanRefer.
\end{enumerate}
\subsection{Context Paragraph}

In the context paragraph, we provided a detailed explanation of the task at hand to the LLM. 
Specifically, we provide context for Gemini to augment the existing ScanRefer description by considering the presence of additional pointing gestures. 
The following phrase was used as the context paragraph.

% \par{\emph{There is a scene where a \variable{HUMAN} is pointing at a \variable{TARGET OBJECT}. 
% There is an external \variable{DESCRIPTION\hey{description of what?}} of the target object which was given to POINT AT \hey{why is this capitalized?} the \variable{TARGET OBJECT} in case the human was not present. 
% Assume that you are that human. 
% What would you say to point at the object while doing the pointing gesture?}}

\emph{There is a scene where a human is pointing at a target object. 
There is an external description of the target object which was given to point at the target object in case the human was not present. Assume that you are that human. What would you say to point at the object while doing the pointing gesture?}

Some examples of queries provided to Gemini are presented in Section~\ref{subsec:prompts}.

% Here are some examples of the context paragraph that we provided to Gemini:
% \begin{itemize}
%     \item \hey{please add real examples here}
% \end{itemize}

\subsection{Output Specifications}

We then provide the LLM with specific instructions on how to structure its response using the following prompt.

\par{
\emph{
Give special attention to the following while answering:
\begin{enumerate}
    \item There may be multiple objects of the same class as the target object.
    \item The human is pointing at the target object.
    \item Do not add information that can not be directly inferred from the query.
    \item Give any 3 possible distinct expressions and no other text.
    \item Do not use any special characters or punctuation marks other than period and comma.
    \item The output format is as follows:
        \begin{enumerate}[a]
            \item Output 1
            \item Output 2
            \item Output 3
        \end{enumerate}
\end{enumerate}
}
}

\subsection{Query}

To guide Gemini in generating a language description that incorporates the presence of pointing gestures, we referenced the existing queries in the original ScanRefer dataset \cite{chen2020scanrefer}. The approach involves taking these original queries and augmenting them to include considerations for an additional pointing gesture in the generated language descriptions.

Here are some examples of queries from the existing ScanRefer dataset:
\begin{itemize}
    \item A black TV, in the direction from the entrance and from the outside, will be on the right side of the blue curtain . on the left of the tv is a small bike.
    \item There is a beige wooden working table. placed on the side of the room
\end{itemize}
%\emph{CURRENT QUERY:\{ScanRefer Query\}}

\subsection{Complete Textual Prompt}

The following shows the complete textual prompt format that was used as an input to Gemini.

\par{\emph{
There is a scene where a human is pointing at a target object. There is an external description of the target object which was given to point at the target object in case the human was not present. Assume that you are that human. What would you say to point at the object while doing the pointing gesture?
\\
}}

\par{\emph{
Give special attention to the following while answering:
\begin{enumerate}
    \item There may be multiple objects of the same class as the target object.
    \item The human is pointing at the target object.
    \item Do not add information that can not be directly inferred from the query. 
    \item Give any 3 possible distinct expressions and no other text.
    \item Do not use any special characters or punctuation marks other than period and comma.
    \item The output format is as follows:
        \begin{enumerate}[a]
            \item Output 1
            \item Output 2
            \item Output 3
        \end{enumerate}
\end{enumerate}
}}

\emph{CURRENT QUERY:\variable{ScanRefer Query}}

\subsection{Some Example Prompts}\label{subsec:prompts}
\subsubsection{Example 1}
\textbf{Prompt to the Gemini:}

There is a scene where a human is pointing at a target object. 
There is an external description of the target object which was given to point at the target object in case the human was not present. Assume that you are that human. What would you say to point at the object while doing the pointing gesture?

Give special attention to the following while answering:
\begin{enumerate}
    \item There may be multiple objects of the same class as the target object.
    \item The human is pointing at the target object.
    \item Do not add information that can not be directly inferred from the query.
    \item Give any 3 possible distinct expressions and no other text.
    \item Do not use any special characters or punctuation marks other than period and comma.
    \item The output format is as follows:
        \begin{enumerate}[a]
            \item Output 1
            \item Output 2
            \item Output 3
        \end{enumerate}
\end{enumerate}

CURRENT QUERY: A black TV, in the direction from the entrance and from the outside, will be on the right side of the blue curtain . on the left of the tv is a small bike.\\

\noindent \textbf{Response from Gemini:}
\begin{enumerate}
    \item That black TV there
    \item The television set to your right
    \item The black TV over there
\end{enumerate}

\subsubsection{Example 2}
\textbf{Prompt to the Gemini:}

There is a scene where a human is pointing at a target object. 
There is an external description of the target object which was given to point at the target object in case the human was not present. Assume that you are that human. What would you say to point at the object while doing the pointing gesture?

Give special attention to the following while answering:
\begin{enumerate}
    \item There may be multiple objects of the same class as the target object.
    \item The human is pointing at the target object.
    \item Do not add information that can not be directly inferred from the query.
    \item Give any 3 possible distinct expressions and no other text.
    \item Do not use any special characters or punctuation marks other than period and comma.
    \item The output format is as follows:
        \begin{enumerate}[a]
            \item Output 1
            \item Output 2
            \item Output 3
        \end{enumerate}
\end{enumerate}

CURRENT QUERY: There is a beige wooden working table. placed on the side of the room.\\

\noindent \textbf{Response from Gemini:}
\begin{enumerate}
        \item The wooden table over there.
        \item The beige table in the corner.
        \item That wooden table by the wall.\\
\end{enumerate}

\subsection{Observations from the (Re)Generated Referring Expressions:}

We observed that the original descriptions in ScanRefer, which were generally longer in word count, were condensed in the \dataset dataset. Additionally, we noticed an increased use of prepositions such as ``here,'' ``that,'' and ``this,'' indicating that, alongside the verbal descriptions, there is also a reliance on pointing gestures to identify the target object.

% \begin{itemize}

% \item \textbf{CURRENT QUERY:}
%     a black tv, in the direction from the entrance and from the outside, will be on the right side of the blue curtain . on the left of the tv is a small bike. \hey{this does not match the format mentioned in A.1.}

%     \textbf{RESULTS:}
%     \begin{enumerate}
%         \item That black TV there
%         \item The television set to your right
%         \item The black TV over there
%     \end{enumerate}
    
% \item \textbf{CURRENT QUERY:} 
%     there is a beige wooden working table. placed on the side of the room.

%     \textbf{RESULTS:}
%     \begin{enumerate}
%         \item The wooden table over there.
%         \item The beige table in the corner.
%         \item That wooden table by the wall.
%     \end{enumerate}
    
% \end{itemize}

\begin{figure}[t]
    \centering
    \includegraphics[width=\linewidth]{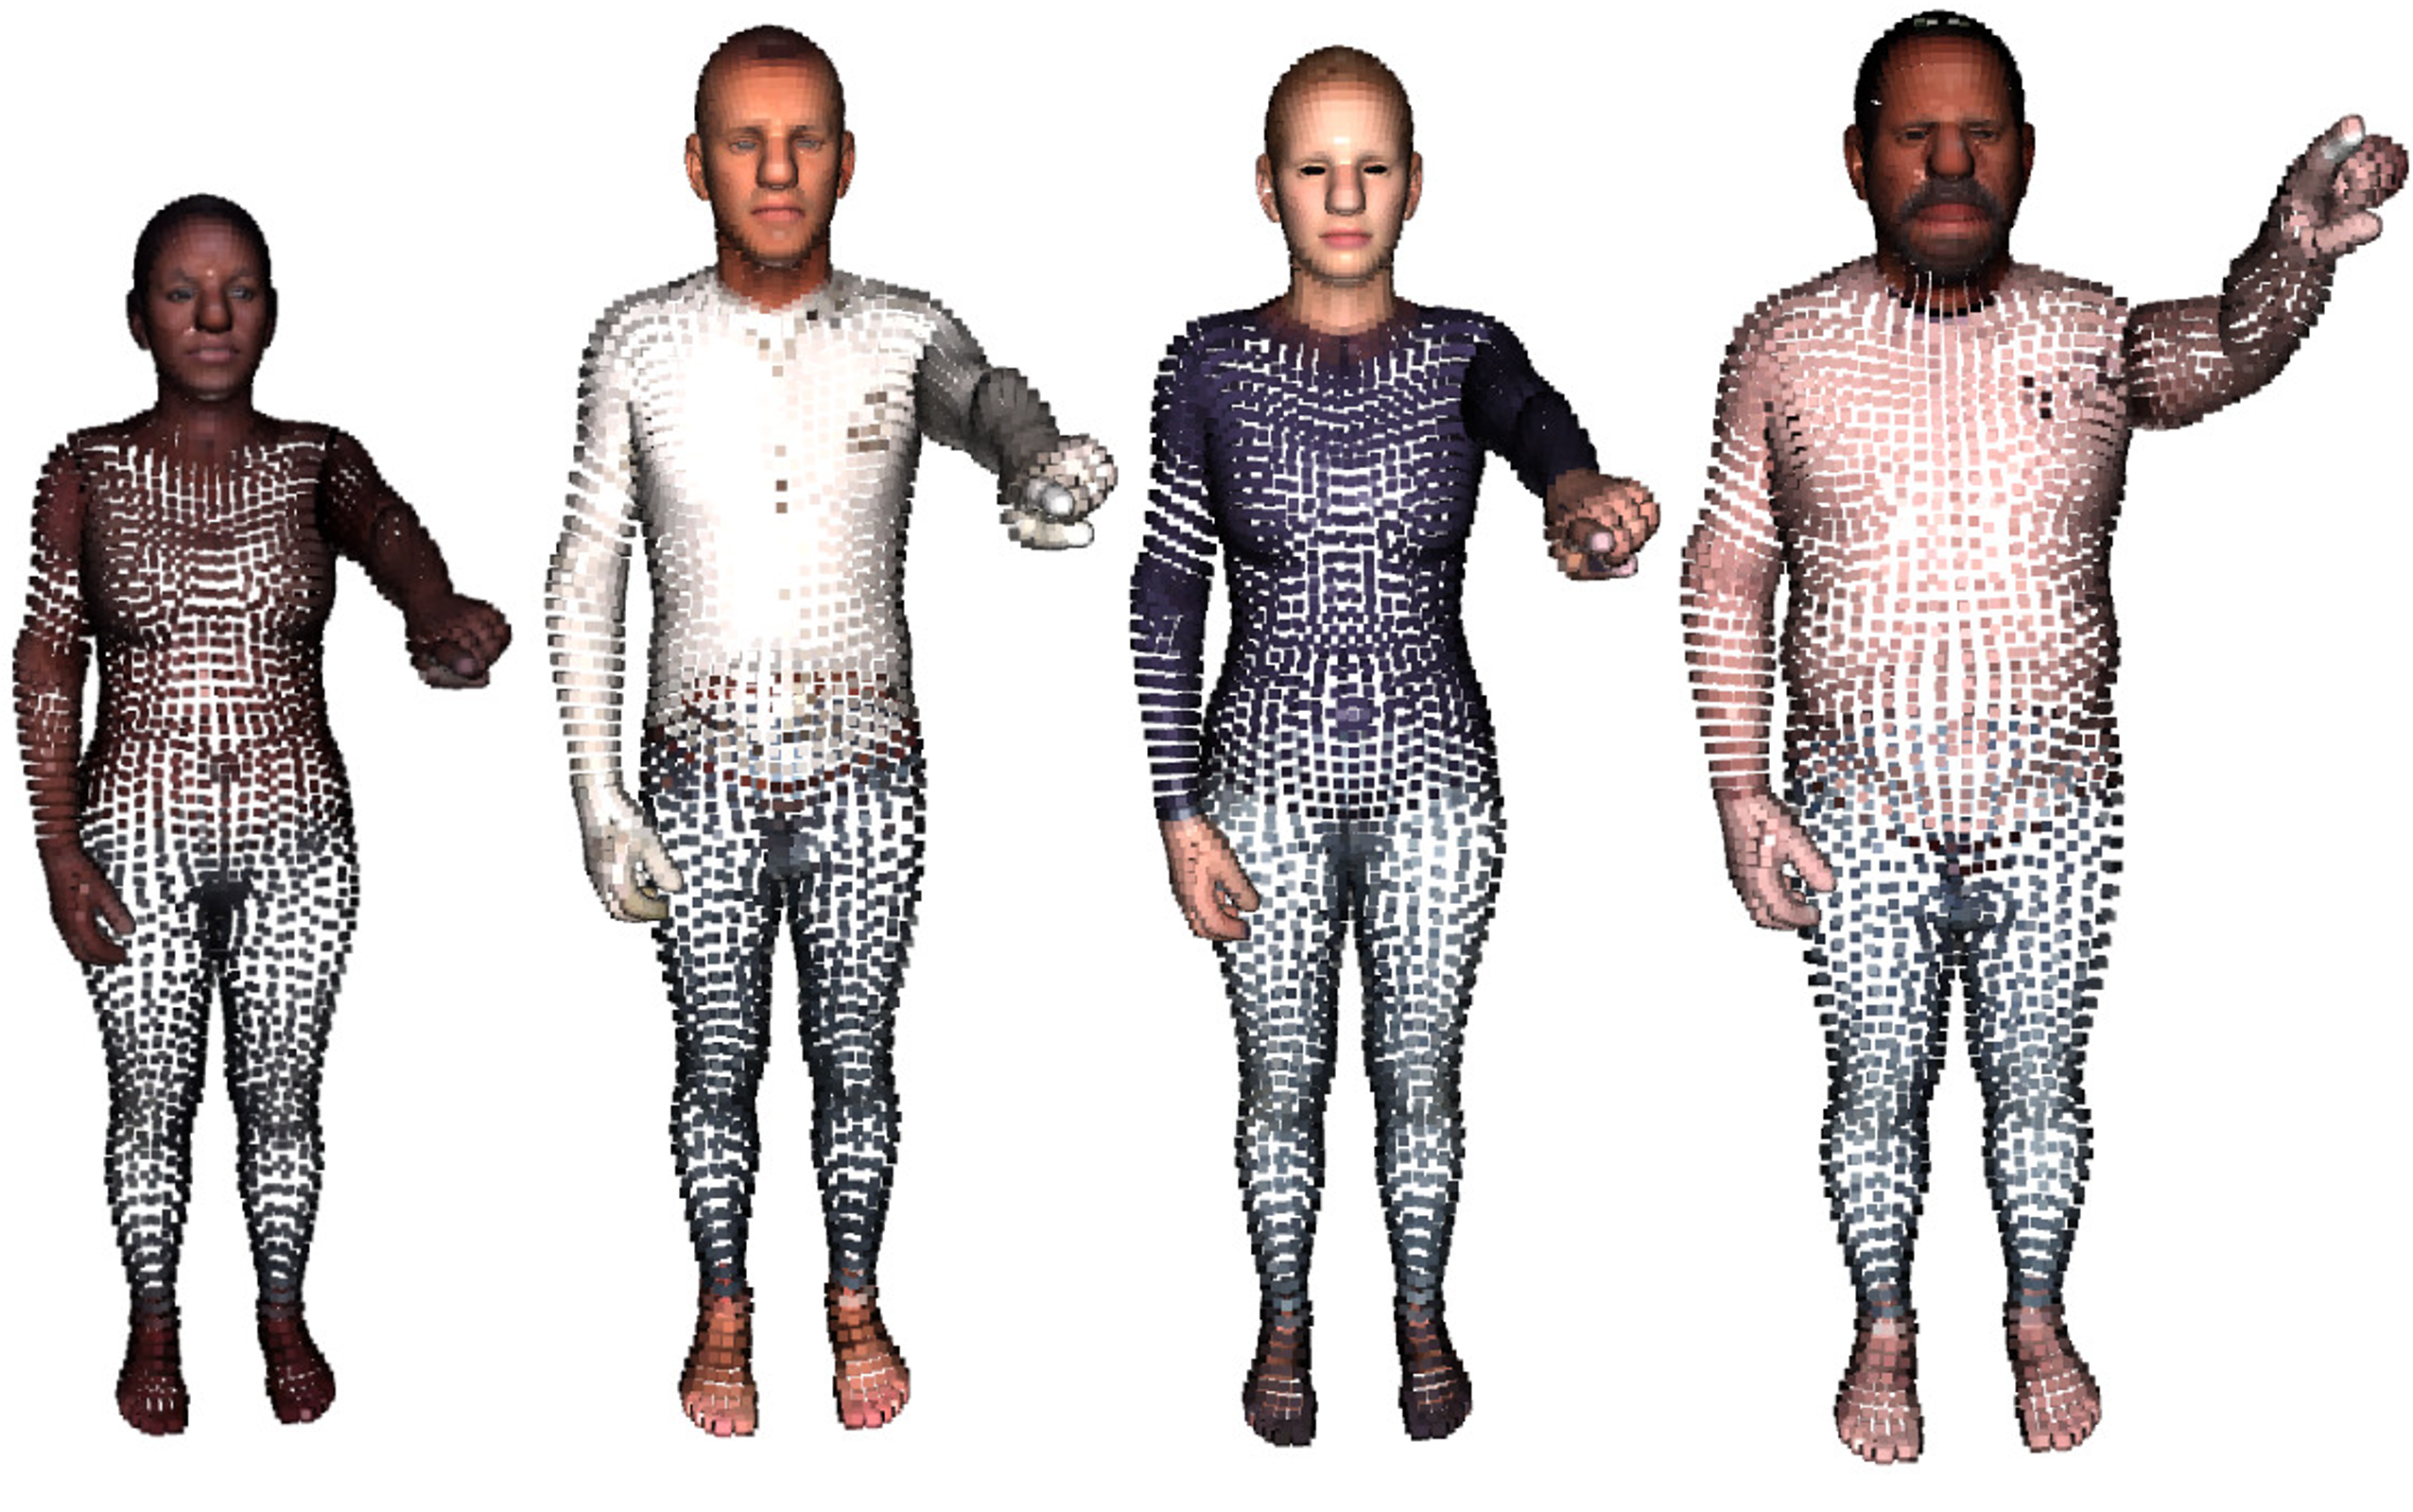}
    \caption{Human avatars used in \dataset dataset.}
    \label{fig:humanAvatars}
\end{figure}

\begin{figure}
    \centering
    \includegraphics[width=0.99\linewidth]{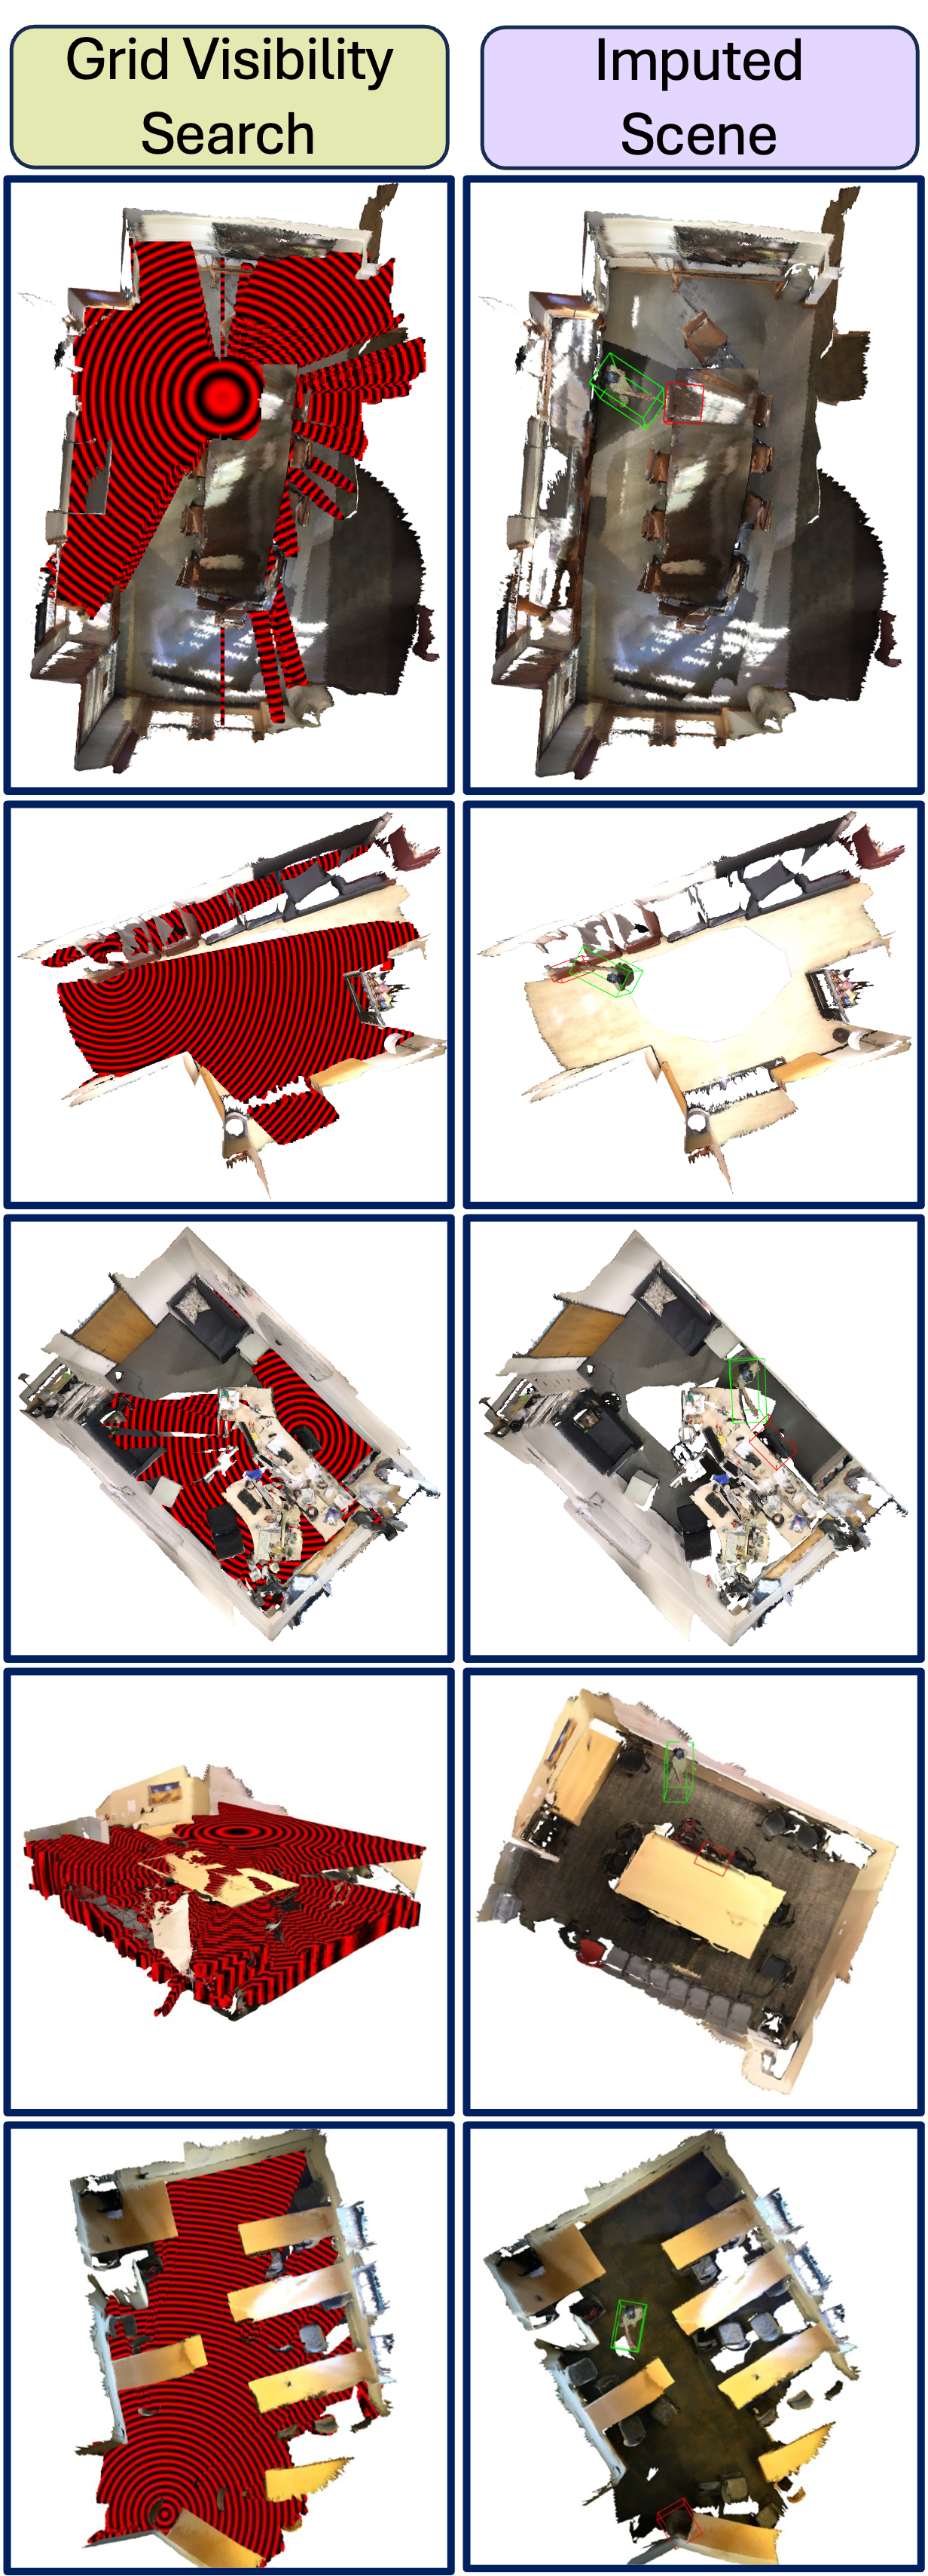}
    \caption{Examples of Imputer Framework}
    \label{fig:exImputer}
\end{figure}

\begin{figure*}[ht]
    \centering
    \begin{subfigure}[b]{0.49\linewidth}
        \centering
        \includegraphics[width=\linewidth]{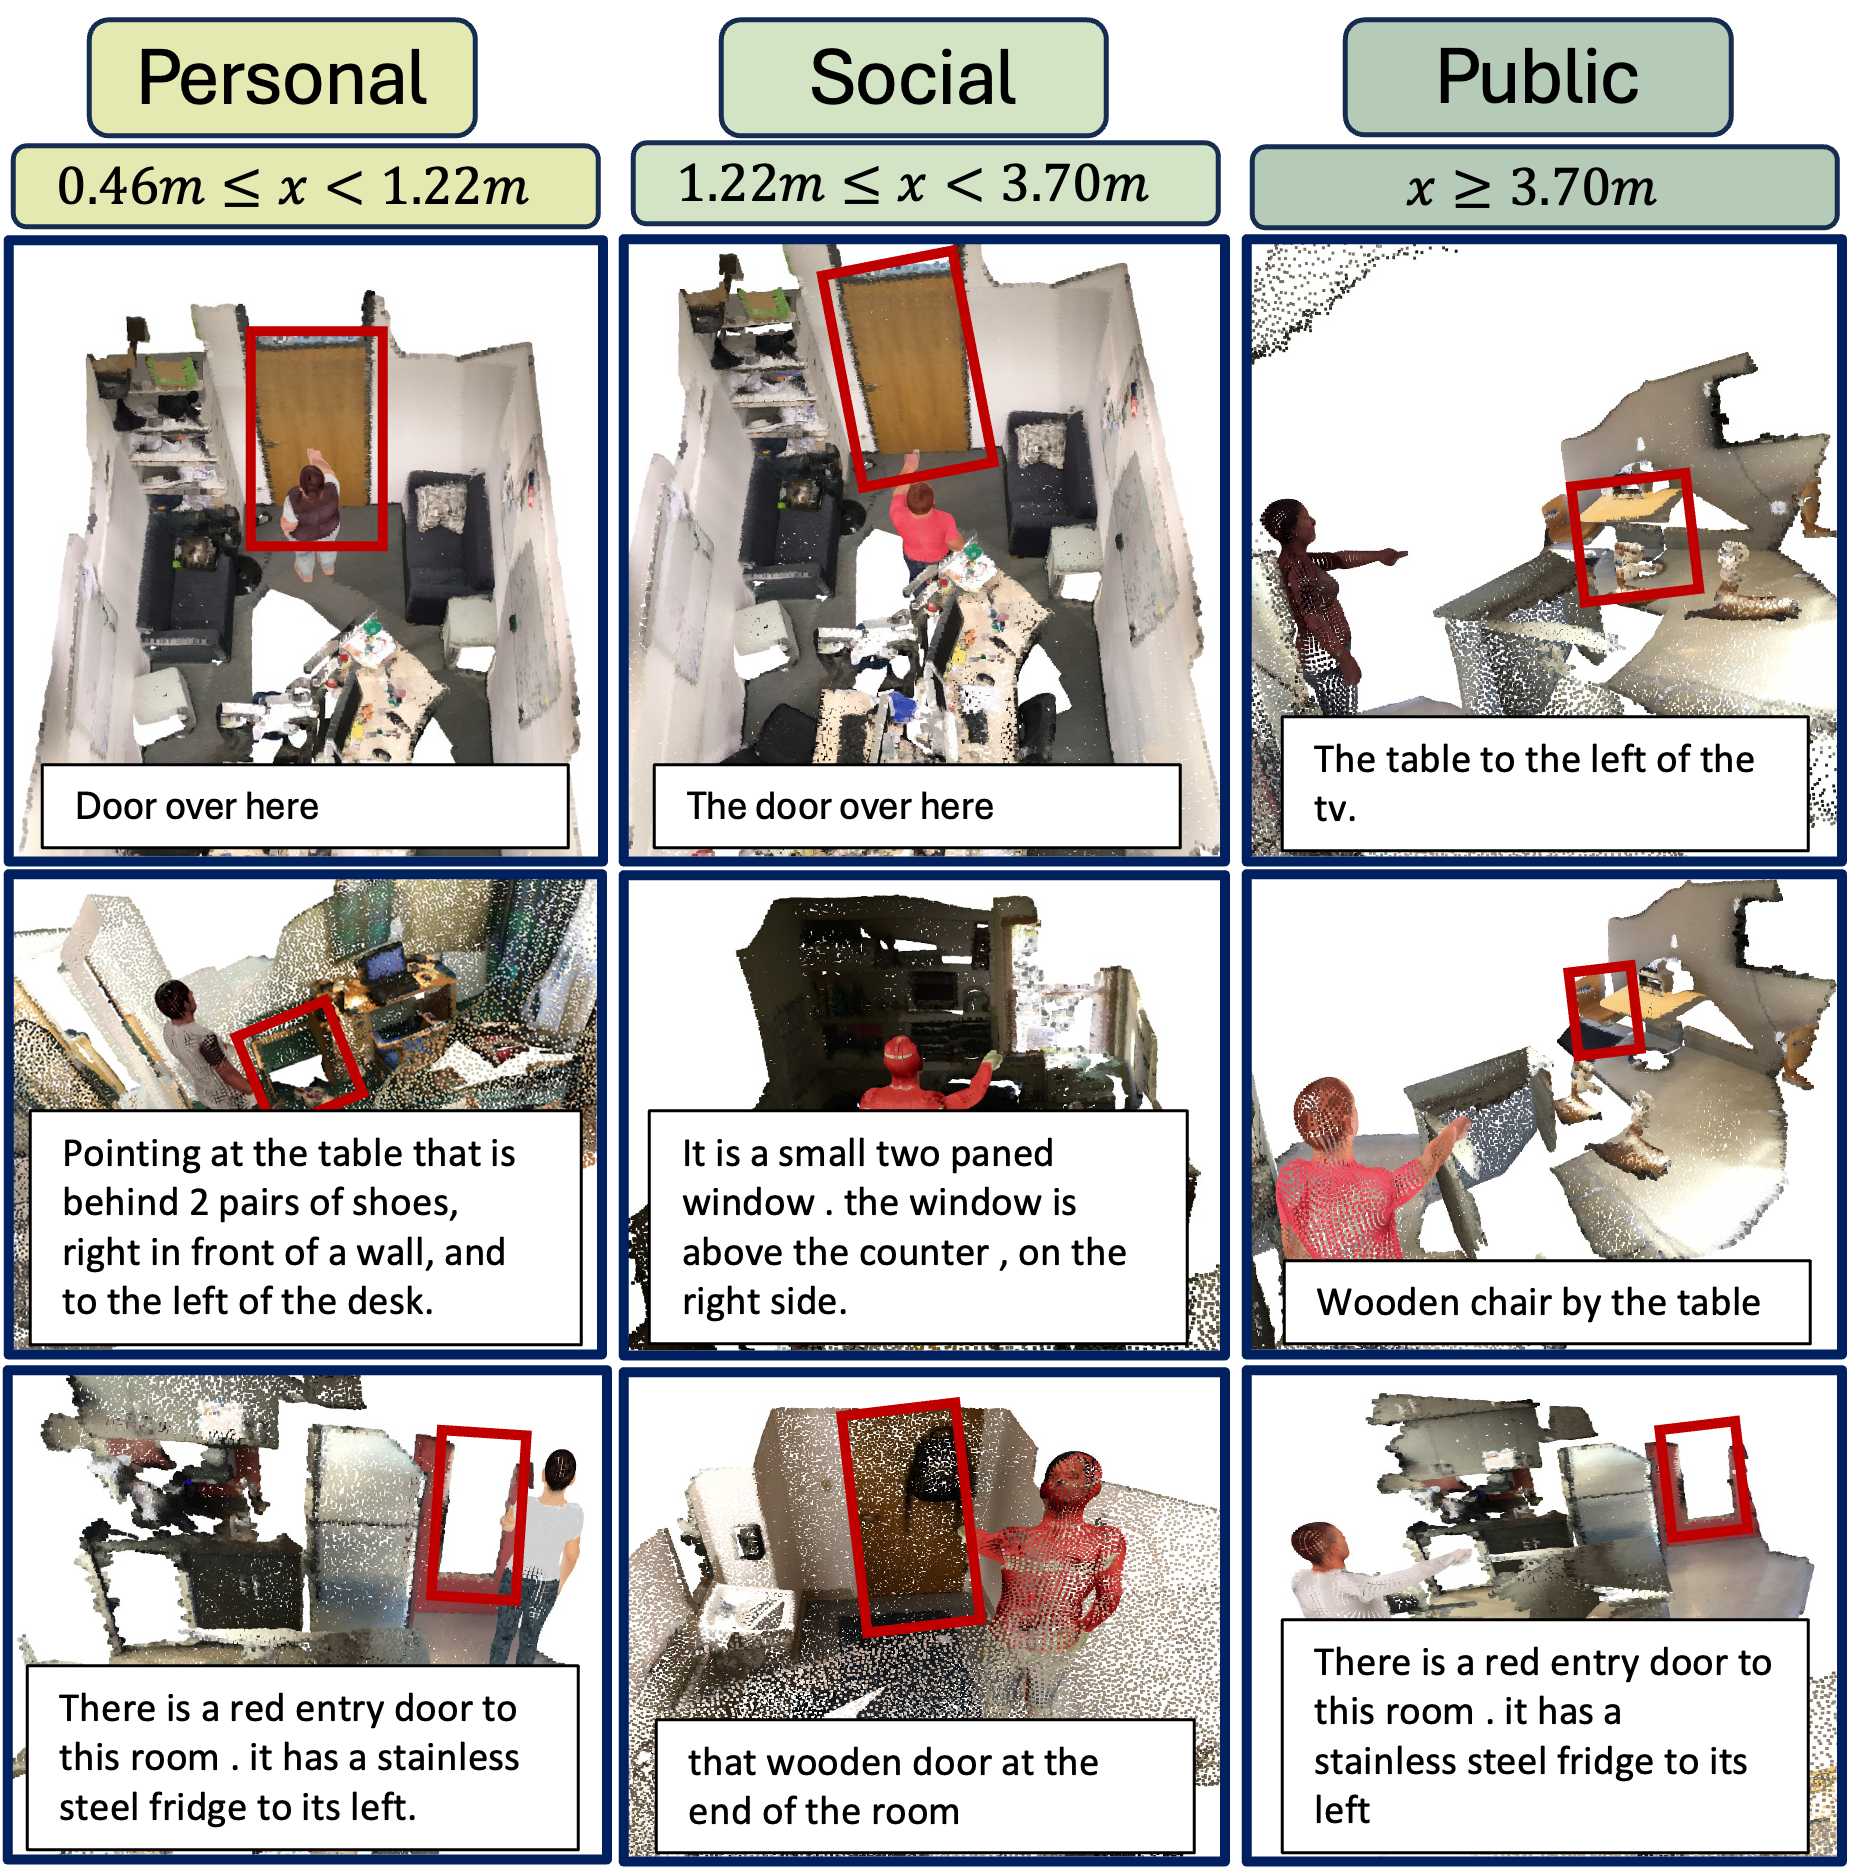}
        \caption{Samples from \dataset with `unique' object scenes}
        \label{fig:unique-set}
    \end{subfigure}
    \hfill
    \begin{subfigure}[b]{0.49\linewidth}
        \centering
        \includegraphics[width=\linewidth]{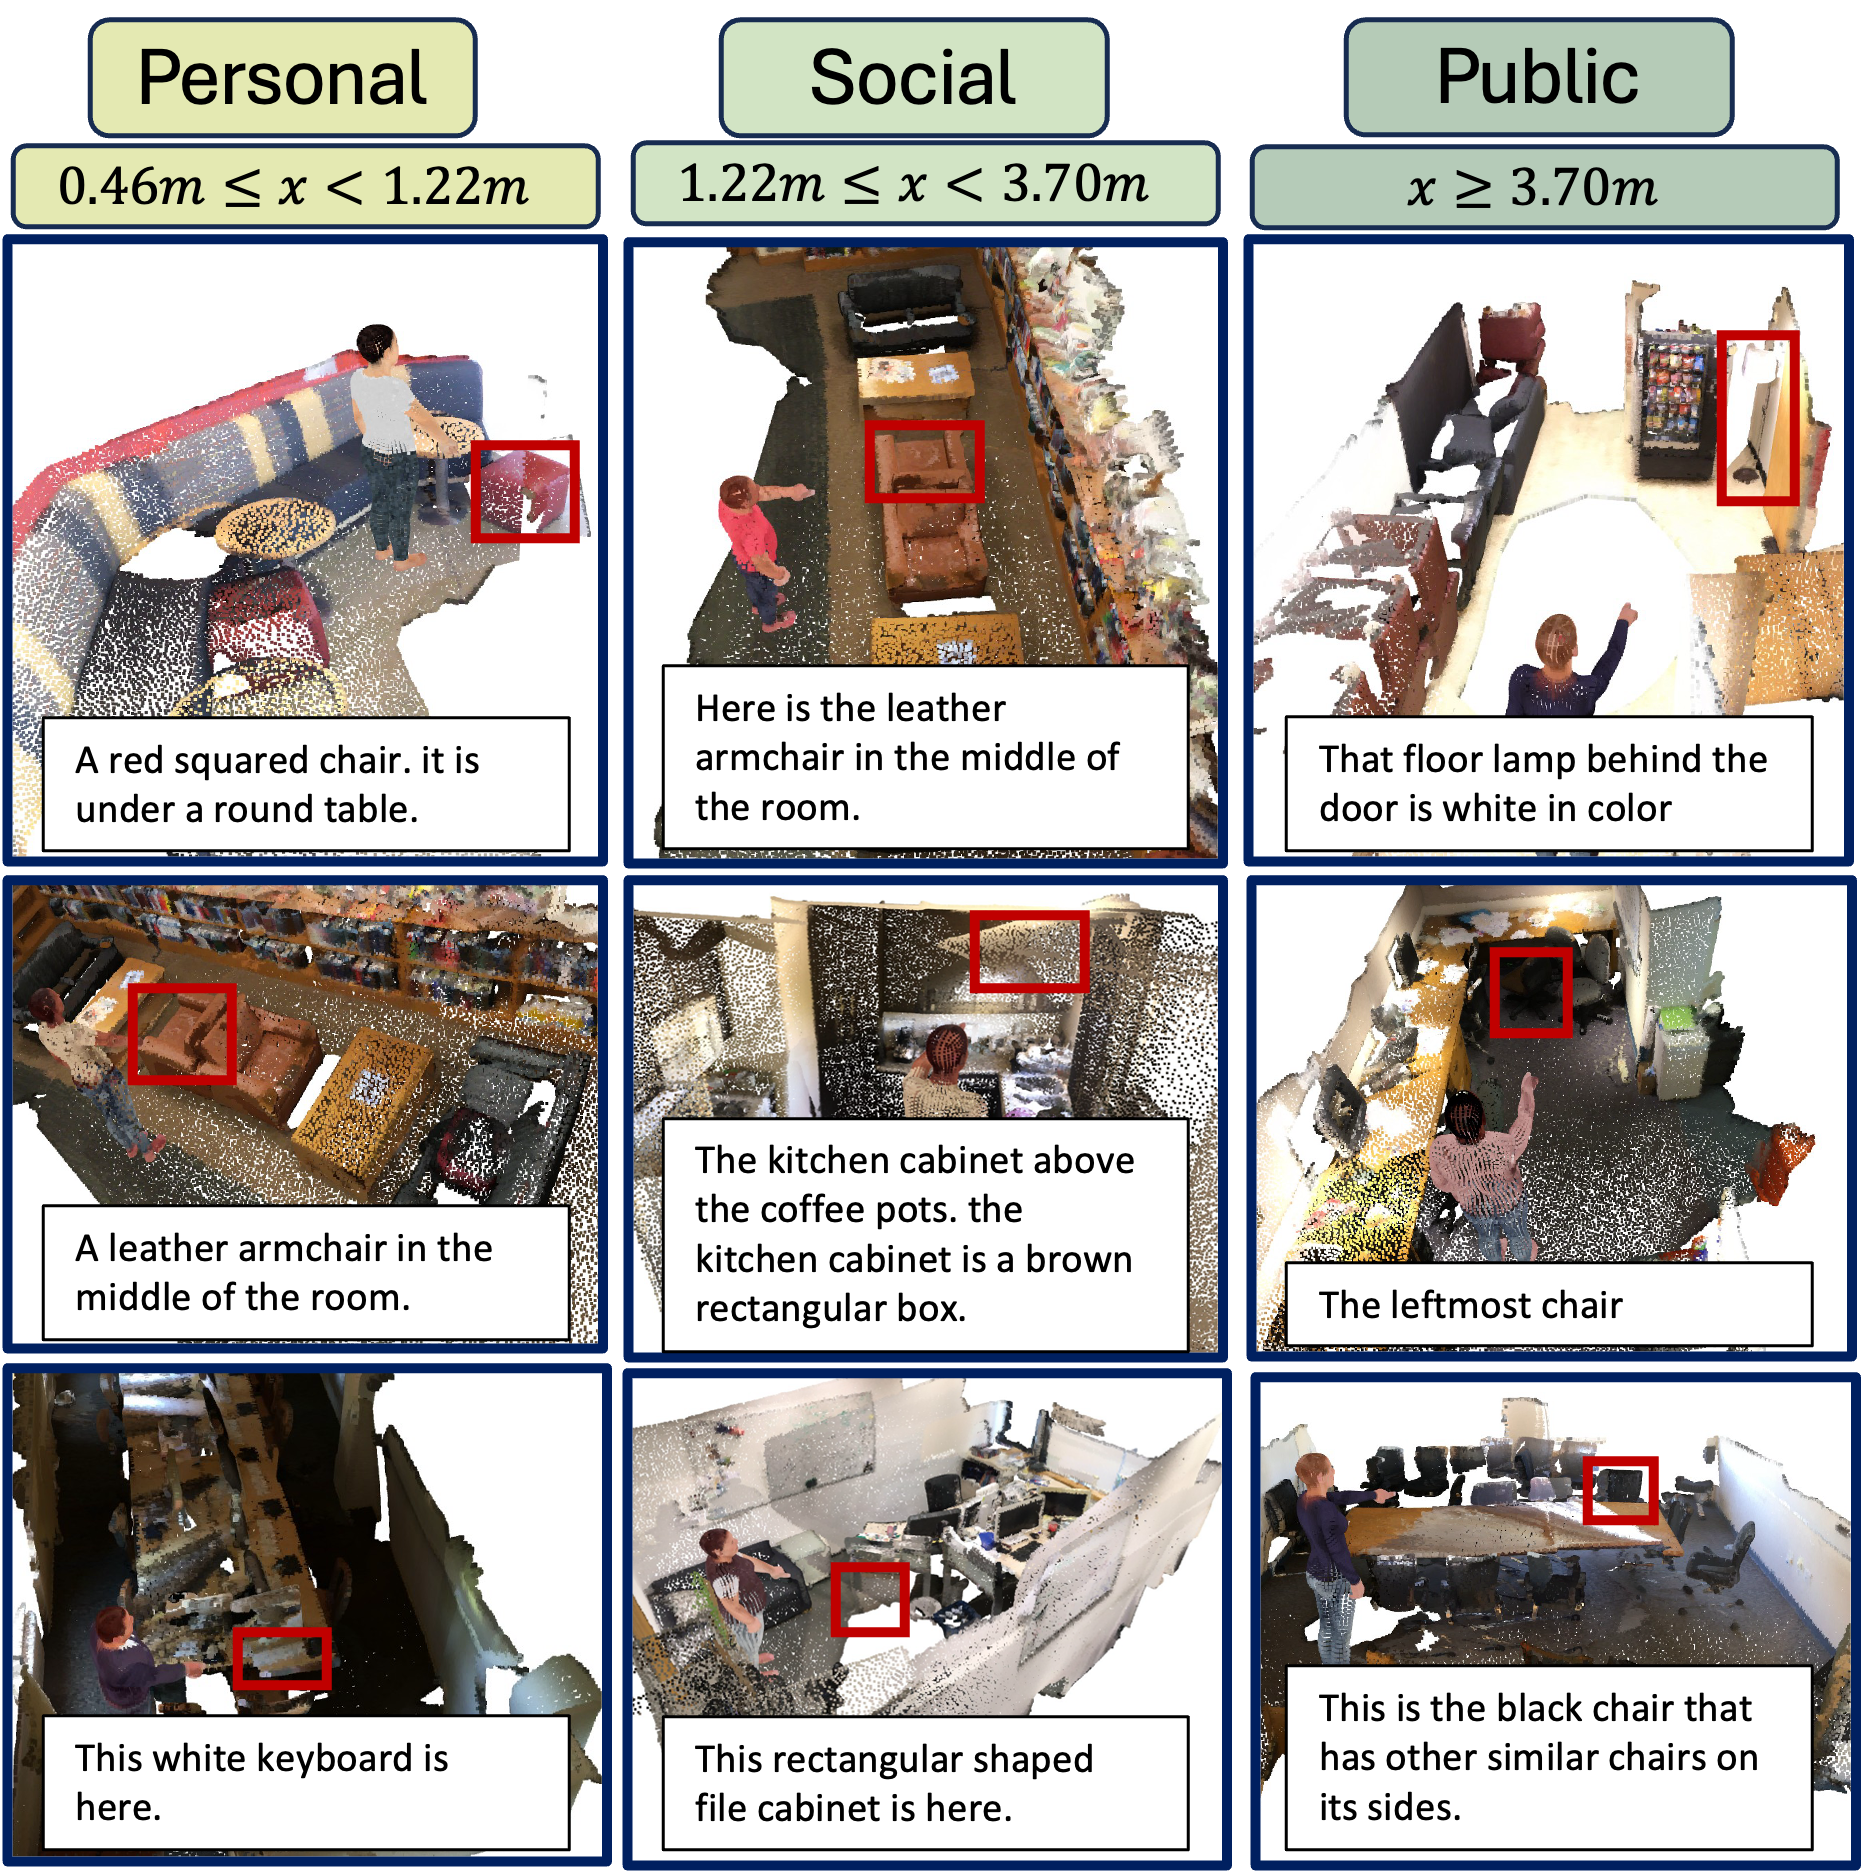}
        \caption{Samples from \dataset with `multiple' object scenes}
        \label{fig:multiple-set}
    \end{subfigure}
    \caption{Samples from \dataset dataset. The imputed human is placed at different distances from the target}
    \label{fig:combined-figure}
\end{figure*}

\section{Example Generations from Imputer}
As described in Section~\ref{sec:pointing-ges-gen}, and presented in Figure~\ref{fig:imputer_fig}, to generate the \dataset dataset, we used multiple human avatars. %\sou{Fig nit referenced}
We present examples of the human avatars used in Figure~\ref{fig:humanAvatars}. In the complete \dataset dataset, we ensure that it is balanced in terms of gender, height, and body mass.

\subsection{Deployment steps for humans in the scene}
Grid visibility search is one of the key intermediate steps of our \aug framework. We showcase additional examples demonstrating the identification of visible regions and the imputation of a human avatar into the existing point-cloud scene in Figure~\ref{fig:exImputer}. In this figure, the images on the left depict the grid-based visibility search used to identify regions with a clear line of sight. The images on the right show the imputed scene after adding the human avatar. The green bounding box highlights the human avatar, while the red bounding box indicates the target object. Visibility values were calculated using the grid-path counting method proposed by Goldstein et al.~\cite{gridwalk}. Regions with visibility values greater than 0.33 and located within the scene were identified as suitable for human imputation, as detailed in the paper.

\subsection{Examples of deployment in Personal, Social, and Public settings for Unique and Multiple objects}
% In the paper we presented one example each of \datasetns for each of the combinations. Here, we present additional examples of scenes, and corresponding query associated with it in each of the scenes. Figure~\ref{fig:unique-set} presents scenes where there is only a unique item placed, and the human avatar is in personal space, i.e., between 0.46~m and 1.22~m. The associated query is also mentioned in the figure. 
% Similarly, Figure~\ref{fig:personalMultiple} presents scenes where there are multiple objects that might be similar to what the query mentions, and the human avatar pointing towards the correct object is within the personal space of the object. 
% We present the social scenarios in Figures~\ref{fig:socialUnique} and~\ref{fig:socialMultiple}, where the avatar is between 1.22~m and 3.70~m of the object of interest.  Figures~\ref{fig:socialUnique} has only one object of interest in the scene, while Figures~\ref{fig:socialMultiple} has multiple objects f interest in the scene. 
% Finally, Figures~\ref{fig:publicUnique} and~\ref{fig:publicMultiple} presents scenes with unique and multiple object of interest respectively, where the distance between the avatar and the object of interest in greater than 3.70~m. 

In the paper, we presented one example from the \dataset for each combination. Here, we provide additional examples of scenes along with the corresponding queries associated with them. Figure~\ref{fig:unique-set} illustrates scenes with `unique' objects, where only one object from the same object class as the target object is present. We include three additional samples that vary based on the distances between the human and the target object: `Personal' (0.46m to 1.22m), `Social' (1.22m to 3.70m), and `Public' (greater than 3.70m).

Similarly, Figure~\ref{fig:multiple-set} illustrates scenes with 'multiple' objects, where there may be more than one object (distractors) belonging to the same class as the target object. As with the 'unique' samples, we provide three additional examples for each distance range.

\begin{table}[]
 \caption{Ablation studies for \names in \dataset dataset} \vspace{-0.1in}
 \label{tab:sup_ablations}
  \resizebox{1.0\columnwidth}{!}{
\begin{tabular}{l|ll|ll|ll}
\hline
\multicolumn{1}{c|}{\multirow{2}{*}{\textbf{Model}}} & \multicolumn{2}{c|}{\textbf{unique}}                                                                                                                                & \multicolumn{2}{c|}{\textbf{multiple}}                                                                                                                              & \multicolumn{2}{c}{\textbf{overall}}                                                                                                                               \\ \cline{2-7} 
\multicolumn{1}{c|}{}                                & \multicolumn{1}{c}{\textbf{\begin{tabular}[c]{@{}c@{}}IoU\\ @0.25\end{tabular}}} & \multicolumn{1}{c|}{\textbf{\begin{tabular}[c]{@{}c@{}}IoU\\ @0.5\end{tabular}}} & \multicolumn{1}{c}{\textbf{\begin{tabular}[c]{@{}c@{}}IoU\\ @0.25\end{tabular}}} & \multicolumn{1}{c|}{\textbf{\begin{tabular}[c]{@{}c@{}}IoU\\ @0.5\end{tabular}}} & \multicolumn{1}{c}{\textbf{\begin{tabular}[c]{@{}c@{}}IoU\\ @0.25\end{tabular}}} & \multicolumn{1}{c}{\textbf{\begin{tabular}[c]{@{}c@{}}IoU\\ @0.5\end{tabular}}} \\ \hline
\names\textsubscript{w/o Gestures}                                         & 69.26                                                                             & 48.84                                                                             & 52.58                                                                             & 37.32                                                                             & 55.79                                                                             & 39.54                                                                            \\
\names\textsubscript{noHumanLoss}                                         & 68.76                                                                             & 48.57                                                                             & 58.75                                                                             & 42.31                                                                             & 60.68                                                                             & 43.51                                                                            \\
%\names\textsubscript{noEF\_noLF}                                         & 62.31                                                                             & 51.99                                                                             & 30.19                                                                             & 24.60                                                                             & 36.38                                                                             & 29.88                                                                            \\
\names\textsubscript{noEF\_onlyLF}                                         & 69.43                                                                             & 49.28                                                                             & 54.81                                                                             & 39.02                                                                             & 57.62                                                                             & 41.00                                                                          \\
\names\textsubscript{onlyEF\_noLF}                                      & 83.71                                                                             & 70.09                                                                             & 66.47                                                                             & 54.92                                                                             & 69.93                                                                             & 58.05                                                                            \\
\names\textsubscript{random\_LF}                                         & 84.0                                                                             & 70.6                                                                             & 66.1                                                                             & 54.6                                                                             & 69.6                                                                             & 57.7                                                                            \\
\names\textsubscript{onlyGest}                                     & 15.29                                                                            & 11.81                                                                            & 12.46                                                                            & 9.80                                                                            & 13.0                                                                            & 10.18                                                                           \\
\names\textsubscript{ConstantLang}                                     & 51.05                                                                            & 43.87                                                                            & 44.89                                                                            & 36.78                                                                            & 46.08                                                                            & 38.15                                                                           \\
\names\textsubscript{GT Poses}                                     & 84.73                                                                            & 71.75                                                                            & 67.99                                                                            & 55.89                                                                            & 70.97                                                                            & 58.99                                                                           \\
\textbf{\names}                                & \textbf{84.60}                                                                             & \textbf{71.03}                                                                             & \textbf{67.57}                                                                             & \textbf{55.77}                                                                             & \textbf{70.85}                                                                             & \textbf{58.71}                                                                            \\ \hline
\end{tabular}
}
\vspace{-0.2in}
\end{table}

\begin{figure}
    \begin{subfigure}{0.49\linewidth}
            \centering
            \includegraphics[width=\linewidth]{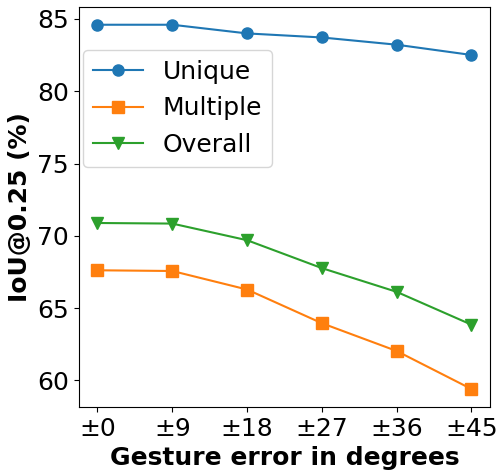}
            \caption{IoU@0.25 (\%)}
            \vspace{-0.1in}
            \label{fig:imprecise_ges_vs_acc25_multi}
        \end{subfigure}
        \hfill
        \begin{subfigure}{0.49\linewidth}
            \centering
            \includegraphics[width=\linewidth]{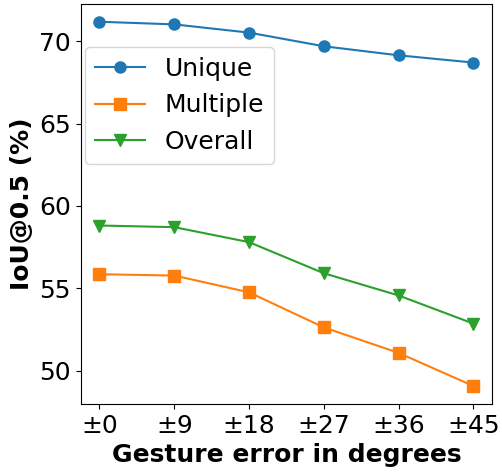}
            \caption{IoU@0.5 (\%)}
            \vspace{-0.1in}
            \label{fig:imprecise_ges_vs_acc50_multi}
        \end{subfigure}%
        
        \caption{Accuracy for multiple vs unique samples for 3D-ERU with imprecise pointing of the human avatar}
        \label{fig:imprecise_ges_multi}
        \vspace{-0.2in}
\end{figure}

\begin{figure}
    \begin{subfigure}{0.49\linewidth}
            \centering
            \includegraphics[width=\linewidth]{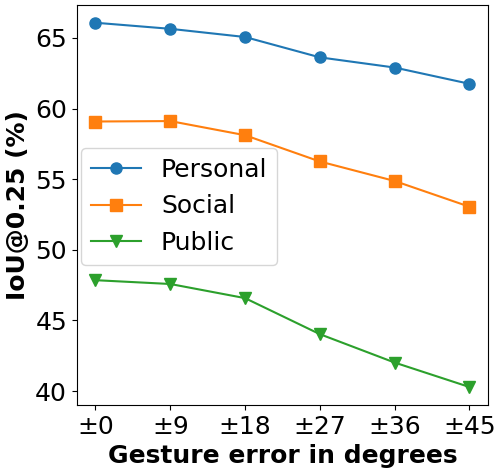}
            \caption{IoU@0.25 (\%)}
            \vspace{-0.1in}
            \label{fig:imprecise_ges_vs_acc25_dist}
        \end{subfigure}
        \hfill
        \begin{subfigure}{0.49\linewidth}
            \centering
            \includegraphics[width=\linewidth]{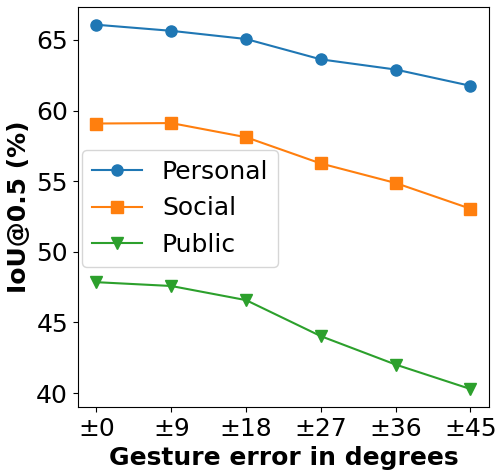}
            \caption{IoU@0.5 (\%)}
            \vspace{-0.1in}
            \label{fig:imprecise_ges_vs_acc50_dist}
        \end{subfigure}%
        
        \caption{Accuracy at different distance ranges for 3D-ERU with imprecise pointing of the human avatar}
        \label{fig:imprecise_ges_dist}
        \vspace{-0.2in}
\end{figure}

\section{Additional Ablation Studies}

We show additional ablation studies in Table \ref{tab:sup_ablations}.
In particular, \names\textsubscript{GT Poses} evaluates the performance of \names when ground truth poses were used for the late fusion instead of the predicted poses from the proposed model. Even when the ground truth pose data is used, \names\textsubscript{GT Poses} saw only a minor boost in accuracy, implying that \names's approach of jointly learning human pose is effective.

As mentioned in Section \ref{sec:method}, we introduced a uniformly sampled rotational jitter ($0 - 9^{\circ}$) in the pointing direction to account for natural human error and variations. In Figure \ref{fig:imprecise_ges_multi} and \ref{fig:imprecise_ges_dist}, we extend this analysis by varying the rotational noise and plotting the resulting accuracy. In Figure \ref{fig:imprecise_ges_multi}, we find that there is only a minor drop in accuracy for the unique object scenarios, even under very high rotational noise. However, for multiple object scenarios, we observe a significant drop in accuracy when rotational noise exceeds $18^{\circ}$. Similarly, from Figure \ref{fig:imprecise_ges_dist}, we see that the drop in accuracy due to imprecise gestures is significant when the human-to-object distance is higher (public distance). Thus, we find that the effect of imprecise gestures is more pronounced at larger distances and in the presence of multiple similar objects. In general, these figures show that \names is able to tolerate rotational noise of up to $18^{\circ}$, reasonably well. A rotational error beyond this range can be deemed infrequent in practical situations.
%\sou{One last sentence mentioning what is implication.... "This shows that Ges3Vig is capable of....."}
